# Supplementary material for: Non-Iterative Disentangled Unitary Coupled-Cluster based on Lie-algebraic structure
Source: arXiv:2408.14289 ancillary file (2025-01-21)
Supplement: Supplementary file 1 [file Revised_NIDUCC_VQE-SI.pdf]

# Supplementary Materials: Non-Iterative Disentangled Unitary Coupled-Cluster based on Lie-algebraic structure

Mohammad Haidar,[1] Olivier Adjoua,[2] Siwar Baddredine,[2] Alberto Peruzzo,[1] and Jean-Philip Piquemal[1,2]

[1] *Qubit Pharmaceuticals, Advanced Research Department, 75014, Paris*[*]

[2] *Sorbonne Université, Laboratoire de Chimie Théorique, UMR 7616 CNRS, 75005, Paris, France*

The Supplementary Materials are organized as follows: Section S1, presents the explicit equations for the second quantized electronic structure Hamiltonian, including the one-body and two-body integrals. Section S2, offers a detailed algorithmic outline of the NI-DUCC-VQE algorithm. Section S3, provides Table S1, which includes resource estimations for NI-DUCC-VQE, UsCCSDTQ-VQE, and ADAPT-VQE (along with their recent versions). Section S4, provides a detailed explanation of the generation process for a Symmetry-Preserving Minimal Complete Pool (MCP), including its definition and key properties. Figures S2 and S3 illustrate the MCP and the product group generations, respectively. Subsection S4A, gives examples of enforcing symmetries on qubit excitations to generate starters for MCP in the $BeH_2$ molecule. Section S5, discusses the differences between Python and C++ implementations for the MCP generations. Figures S3(a) and S3(b) illustrate how the construction of the MCP scales with the number of qubits, focusing on both memory usage and computational time. Sections S4 and S5 complement the discussion in Section IV.B of the main text.

## 1. ELECTRONIC STRUCTURE HAMILTONIAN IN SECOND QUANTIZATION FORMALISM

In the context of quantum chemistry, the Hamiltonian is expressed in the fermionic second-quantization form [1]:

$$\hat{H} = \sum_{i,j=1}^{n} h_{ij} c_i^\dagger c_j + \frac{1}{2} \sum_{i,j,k,l=1}^{n} v_{ijkl} c_i^\dagger c_j^\dagger c_k c_l \tag{1}$$

where $\hat{c}_i^\dagger$ ($\hat{c}_j$) are anti-commuting operators that create (annihilate) electrons in molecular spin-orbital $i(j)$, respectively. The symbols $h_{ij}$ and $v_{ijkl}$ are the one and two electron integrals. The one-electron integrals are obtained from the kinetic energy and electron-nuclei interactions, while the two-electron integrals are obtained from the electron-electron interactions, and are computed in the basis set $\{\chi_i(\vec{\mathbf{x}})\}_{i=1}^n$, given as

$$h_{ij} = \int_{\mathbb{R}^3} d\vec{\mathbf{x}}\, \chi_i^*(\vec{\mathbf{x}}) \left( -\frac{\nabla^2}{2} - \sum_A \frac{Z_A}{r_{A\vec{\mathbf{x}}}} \right) \chi_j(\vec{\mathbf{x}}) \tag{2}$$

and

$$v_{ijkl} = \int_{\mathbb{R}^3} \int_{\mathbb{R}^3} d\vec{\mathbf{x}}_1 d\vec{\mathbf{x}}_2 \frac{\chi_i^*(\vec{\mathbf{x}}_1)\, \chi_j^*(\vec{\mathbf{x}}_2)\, \chi_k(\vec{\mathbf{x}}_1)\, \chi_l(\vec{\mathbf{x}}_2)}{r_{12}} \tag{3}$$

By selecting Gaussian single-particle basis functions, these two integrals (2) and (3) are efficiently commutable on classical computer. In equation (2), $\nabla^2$ is the Laplacian operator with respect to the electronic spatial coordinates. The positive scalar $r_{A\vec{\mathbf{x}}}$ is the Euclidean distance between the $A^{th}$ nucleus and the electron, while $r_{12}$ is the Euclidean distance between two electrons. In both equations (2) and (3), the spin of the electron can be integrated out, resulting in integrals over the spatial components.

---

* Mohammad.haidar@qubit-pharmaceuticals.com; alberto.peruzzo@qubit-pharmaceuticals.com; jean-philip.piquemal@sorbonne-universite.fr

## 2. NI-DUCC-VQE ALGORITHM

**Algorithm 1:** NI-DUCC-VQE

```
D ← Generate all double excitations (i, j, k, l) of UCCSD;
v ← Determine the electronic Hamiltonian matrix elements connecting the spin orbitals involved in double
    excitations ;
t ← Initialize a zeros array, which corresponds to the parameters of the double excitation operators
// Step1: Select dominant sparse operators
A ← Empty List;
for ε ∈ {10^-1, 10^-3, 10^-4} do
    for each (i, j, k, l) ∈ D do
        if max(v_ijkl, t_ijkl) > ε then
            Append (i, j, k, l) to A
        end
    end
    Update t ← VQE(A);
end

// Step2: Filter operators and convert to qubit excitations
for each (i, j, k, l) ∈ A do
    if EvenY(i, j, k, l) or BreaksNumber(i, j, k, l) or
       BreaksSpin(i, j, k, l) or BreaksSpatial(i, j, k, l) then
        Remove (i, j, k, l) from A
    end
end
// Strongly Correlated Starters (SCS)
SCS ← A;
// Step3: Generate Minimal Complete Pool
MCP ← GenerateMCP(SCS);
// Step4: Optimize the Parameters
// Choose repeater k
Choose k layers;
kMCP ← Extend(MCP, (k-1)SCS);
Apply VQE(kMCP)
```

## 3. RESOURCES ESTIMATIONS NI-DUCC-VQE VS USCCSDTQ-VQE VS ADAPT-VQE

| **Method** | Bound | **Gradient** | **Parameter** | **CNOT** |
|---|---|---|---|---|
| Fermionic-AD-VQE [2] | threshold to (iter = $N_s$) | $\mathcal{O}(n^8)$ | $\mathcal{O}(N_s)$ | $\mathcal{O}(n_f(S,D)N_s)$ |
| Qubit-AD-VQE [3] | threshold to (iter = $N_s$) | $\mathcal{O}(n^8)$ | $\mathcal{O}(N_s)$ | $\mathcal{O}(n_q(S,D)N_s)$ |
| QEB-AD-VQE [4] | threshold to (iter = $N_s$) | $\mathcal{O}(n^8)$ | $\mathcal{O}(N_s)$ | $\mathcal{O}(n_{qexc}(S,D)N_s)$ |
| ADAPT-RDM-VQE [5] | threshold to (iter = $N_s$) | $\mathcal{O}(n^6)$ | $\mathcal{O}(N_s)$ | $\mathcal{O}(n_f(S,D)N_s)$ |
| ADAPT-V-VQE [5] | threshold to (iter = $N_s$) | $\mathcal{O}(n^5;n^8)$ | $\mathcal{O}(N_s)$ | $\mathcal{O}(n_f(S,D)N_s)$ |
| ADAPT-VX-VQE [5] | threshold to (iter = $N_s$) | $\mathcal{O}(n^4)$ | $\mathcal{O}(N_s)$ | $\mathcal{O}(n_f(S,D)N_s)$ |
| TETRIS-ADAPT-VQE [6] | threshold to (iter = $N_s$) | $\mathcal{O}(n^5;n^8)$ | $\mathcal{O}(N_s)$ | $\mathcal{O}(n_{qexc}(S,D)N_s)$ |
| Sym-qubit-ADAPT-VQE [7] | threshold to (iter = $N_s$) | $\mathcal{O}(n^5)$ | $\mathcal{O}(N_s)$ | $\mathcal{O}(pN_s)$ |
| Overlap-ADAPT-VQE [8] | threshold to (iter = $N_s$) | $\mathcal{O}(n^5;n^8)$ | $\mathcal{O}(N_s)$ | $\mathcal{O}(n_{qexc}(S,D)N_s)$ |
| UsCCSDTQ-VQE [9] | threshold to (iter = $N_s$) | None | $\mathcal{O}(n_{ops})$ | $\mathcal{O}(n_f(S,D,T,Q)N_s)$ |
| COMPASS-VQE [10] | threshold to (ops = $n_{ops}$) | None | $\mathcal{O}(n_{ops})$ | $\mathcal{O}(n_f(D)n_{ops})$ |
| COMPACT-VQE [11] | threshold to (ops = $n_{ops}$) | None | $\mathcal{O}(n_{ops})$ | $\mathcal{O}(n_f(S,D)n_{ops})$ |
| NI-DUCC-VQE (**This work**) | Lie algebra($n_{set}$) to layers($k$) | None | $\mathcal{O}(kn_{set})$ | $\mathcal{O}(knp)$ |

TABLE S1: Resources estimations involved in implementing the recent ADAPT-VQE algorithmic variants as well as the two fixed ansatz UsCCDSTQ and NI-DUCC-VQE algorithms. $n$ denotes the number of qubits, which corresponds to the number of spin-orbitals; In column 2, the term *Bound* refers to the threshold set in each of the algorithms, for example if the threshold is set to $10^{-5}$ Hartree for an energy reduction purpose, the algorithm *terminates* at this threshold after a certain number of iterations or number of operators, denoted as $N_s$ and $n_{ops}$ respectively. This is why we refer to it as *threshold to iter* = $N_s$. We described in the same way the required conditions for the COMPASS, COMPACT, UsCCSDTQ and NI-DUCC fixed ansätze. In column 3, the term *Gradient* refers to the gradient measurements per one iteration in a VQE process. The total gradient is then the total number of iterations $N_s$ multiplied by the total number of measurements. In NI-DUCC-VQE and UsCCSDTQ-VQE, the gradient is *None*, indicating that residual gradients do not need to be computed, and this is the main distinction from the principles of ADAPT-VQE. In column 3, the notation $\mathcal{O}(n^5;n^8)$, indicates that the gradient calculations range between scales $\mathcal{O}(n^5)$ and $\mathcal{O}(n^8)$. In column 4, *Parameter* denotes the number of parameters present within the ansatz. If ADAPT-VQE ansatz is used, then the number of parameters is equal to the number of iterations $N_s$. When using the UsCCSDTQ, COMPASS and COMPACT ansätze, the number of parameters equals the number of selected operators, $n_{ops}$ as described in the main text. In UsCCSDTQ, $n_{ops}$, are chosen through the fermionic pre-screening process. In the COMPASS approach, the number of operators, $n_{ops}$, is determined using two threshold parameters, $\varepsilon_1$ and $\varepsilon_2$, which ensure the inclusion of the most significant cluster amplitudes and scatterers in the final ansatz. Thus, COMPASS calculations with thresholds $\varepsilon_1$ and $\varepsilon_2$ are denoted as COMPASS($-\log(\varepsilon_1), -\log(\varepsilon_2)$). The COMPACT method uses spin-complementary excitations, where $n_{ops}$ is determined through three thresholds, $\epsilon_1, \epsilon_2$, and $\epsilon_3$, and denoted as COMPACT($-\log(\epsilon_1), -\log(\epsilon_2), -\log(\epsilon_3)$). In contrast, for the NI-DUCC ansatz, the number of parameters corresponds to the product of the number of generators, $n_{set}$ and the number of $k$ layers. Column 4 presents the *CNOT* counts, however, scaling them depends on the type of excitation and method used in the pool: (i) for fermionic excitations, denoted $n_f$, the method "staircase" [12–14] is used, where $n_{Sf} = 4n_S - 4$, $n_{Df} = 16n_D - 16$, $n_{Tf} = 64n_T - 64$ and $n_{Qf} = 256n_Q - 256$, stand for the number of CNOT gates resulting from single, double, triple and quadruple excitations respectively. In these expressions, $n_S$,$n_D$, $n_T$ and $n_Q$ denote the range of qubits involved in each single, double, triple and Quadruple excitations, respectively. (ii) for qubit excitations denoted, $n_q$, we have for each Pauli string of length $p$, a $2p-2$ CNOT counts by using staircase method. (iii) for QEB Qubit excitations, denoted $n_{qexc}$, the method "efficient qubit excitations" [4] is used where each single and double excitations require $n_{Sq} = 2$ and $n_{Dq} = 13$ CNOTs, respectively. Finally the CNOT counts in NI-DUCC ansatz, are computed from the multiplication of the number of layers ($k$) with the number of Pauli string ($2p-2$) and with the number of excitations in the set ($n_{set}$) generated by the symmetry-preserving MCP. The $n_{set}$ scales linearly with the number of qubits $n$, as explained in the main text.

## 4. GENERATION OF A SYMMETRY-PRESERVING MINIMAL COMPLETE POOL (MCP): DEFINITION AND PROPERTIES

In this Section, we summarize the key points, definitions, and properties required to construct a symmetry-preserving minimal and complete pool [7].

The qubit excitation operator pools are defined as sets of anti-Hermitian Pauli strings, $\mathcal{S} = \left\{\hat{P}_k, k \in \{1, \ldots, L\}\right\}$, with $L$ being the size of the pool. $\mathcal{S}$ includes the qubit excitation operators and their commutators. From this set of excitations, one can generate parameterized unitaries defined as

$$\mathcal{S}_g = \left\{\exp(\alpha_k \hat{P}_k), k \in \{1, \ldots, L\}\right\}.$$

The pool $\mathcal{S}$ is said to be *complete*, if for any two states $|\Psi\rangle$ and $|\Phi\rangle$, there exists a product of unitaries from $\mathcal{S}_g$ that transforms one state into another.

The algebra which contains these qubit excitation operators, can transform a qubit state $|000\ldots0\rangle$ to any other state, consists of at least $2^n - 1$ Pauli strings ($2^n$ possible configurations less the vacuum state). Therefore it is possible to create a complete pool consisting of $\mathcal{O}(2^n)$ excitations, where $n$ is the number of qubits. However, as mentioned in the main text, this scale is not desirable. While a wavefunction with "complete" excitations can be constructed, the number of excitations grows exponentially as a function of $n$, which leads to an exponential increase in the number of parameters to optimize. Therefore, selecting an optimal set of generators is essential for constructing a compact wavefunction, which tackles the exponential growth. A minimal and complete pool (MCP) of excitations, as discussed in [7], uses Lie algebraic properties to scale linearly, as $\mathcal{O}(n)$, with the number of qubits. In order to create a complete pool, one needs to follow theorems 1 and 2 given in [7]. This can be summarized as follows (see figure below):

Let $\mathcal{S} = \left\{\hat{P}_k, k \in \{1, \ldots, 2n-2\}\right\}$ be a pool of $2n - 2$ odd Pauli strings. According to the theorems of completeness, as described in [7], this pool must

- **Satisfy the group size criteria** This implies that the size of the product group generated from $S$ should match the size of the product group generated from the pool $G$, which consists of the following elements:

$$G = \{Z_1, Z_2, \ldots, Z_{n-2}, Y_1, Y_2, \ldots, Y_{n-2}, Y_{n-1}, Z_{n-1}Y_n\}.$$

- **Satisfy the inseparability condition.** When constructing the set $\mathcal{S}$, the selected strings should not commute with the previously added strings contained in the pool. This inseparability condition is verified in the fourth step of the MCP generation process, as detailed in the main text (see Section IV.B).

- ***Optional step***. For a fully analytical proof of completeness, one should compute the algebra generated by the elements of $\mathcal{S}$, and ensure that it spans all odd strings from the product group generated from $G$. We restrict ourselves to only elements satisfying the symmetries as explained in 4 A. As a result, the pool generates a subalgebra with "symmetric" odd Pauli strings.

The following scheme S1 is applicable for verifying the completeness conditions of a given pool of Pauli Strings. $\mathcal{G}_{CP}$ represents the product group generated by the set $G$. From $\mathcal{G}_{CP}$, we derive $\mathcal{G}_{FG}$ by selecting only the elements that satisfy both the Parity and EvenFlip symmetries. The final set, $\mathcal{G}_{FS}$, is obtained by further filtering $\mathcal{G}_{FG}$ to include only the Odd Pauli strings. To verify the completeness conditions, one needs to start by generating the product group from the elements in $S$ (which contains symmetric Pauli strings). Subsequently, the three conditions outlined above should be assessed to ensure completeness.

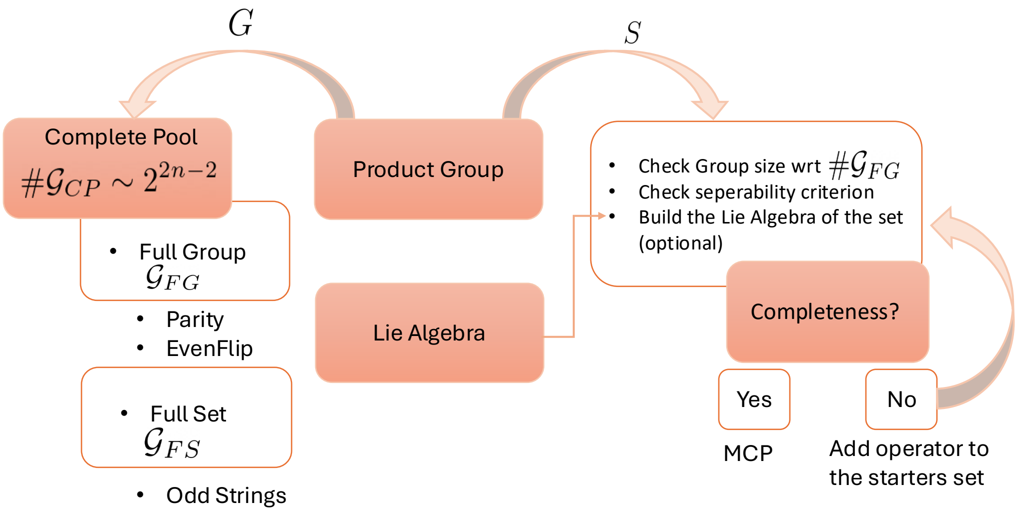


FIG. S1: Sketch for constructing MCP: the theorems and observations outlined above provide a practical method for identifying complete pools. The task is as follows: given a pool set of Pauli strings, determine whether it is complete.

We examine below how the product group is constructed from a given set of Pauli string generators.

Let $\mathcal{S} = \left\{\hat{P}_k, k \in \{1, \ldots, L\}\right\}$ be the set of Pauli string operators, with $L$ being the length of $\mathcal{S}$. Let us define a function $g$ that computes the product of two Pauli strings. For example, consider an 8-qubit system with $\hat{P}_1 = \text{XZIZYZII}$, and $\hat{P}_2 = \text{ZYYXXYXY}$, then

$$g(\hat{P}_1, \hat{P}_2) = \text{YXYYZXXY}\,. \tag{4}$$

The product group generated by $\mathcal{S}$ is illustrated in the following graph, where $\mathcal{S}_0 = \left\{\underbrace{\text{III}\ldots\text{I}}_{n}\right\}$. In this graph, the red solid shapes represent the $k$-th Pauli string in $\mathcal{S}$, denoted as $\hat{P}_k$, for $k \in \{1, \ldots, L\}$. The connecting edges indicate their multiplication with the elements in the previous set $\mathcal{S}_{k-1}$. The results are then appended to $\mathcal{S}_{k-1}$ in order to form the new set $\mathcal{S}_k$, but any existing redundant terms should be removed. One can observe that the size of the set increases exponentially with the added strings, which is the main bottleneck in the computational costs on a classical computer.

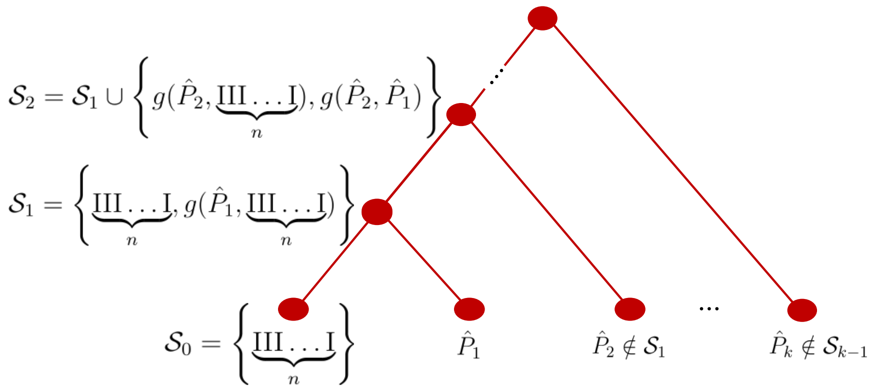


FIG. S2: A sketch illustrating the generation of the product group from a given set of Pauli string operators.

By addressing problems related to the symmetries of the Hamiltonian, one can further reduce computational resources. This can be achieved by focusing on the specific properties of qubit excitations that preserve symmetry and leveraging the inherent properties of the wavefunction. In the following subsection, we demonstrate how to impose different symmetry properties on the excitations, creating what we refer to as "symmetric starters," which are applied on top of the Hartree-Fock state, as discussed in the main text. While this approach is primarily designed for ground-state systems, it can also be extended to excited states or open-shell molecules, with necessary adjustments to the symmetries. For instance, when targeting the first excited state, it is crucial to identify the orbitals specific to that state and apply the corresponding point group symmetry. Since the irreducible representation of the excited state may differ from the ground state, careful attention is needed when applying symmetries such as Total Spin and spin projections. To accommodate excited states, the implemented code (and functions related to the symmetries) will need to be updated accordingly.

### A. Enforcing Symmetries in Qubit Pauli Excitations

- **Odd string**: To make the total wavefunction real, the set of Pauli strings $\left\{\hat{P}_l\right\}_{l=1}^{M}$, with $M$ being the length of the starters set, should include odd total number of Pauli $Y$ matrices. For example, for four qubits, we can have $\hat{P}_l = X_0\,Y_1\,X_2\,X_3$.

- **No More Than Double**. This condition is important to avoid single, triple, quadruple excitations etc. The commutator calculations $[\hat{P}_l, \hat{H}]$ are equal to zero with respect to Hartree-Fock, if and only if $\hat{P}_l$ creates more than double excitations on top of the Hartree-Fock state. This is a consequence of the molecular Hamiltonian containing only single and double excitations. Therefore, it cannot connect, for example, the states 11110000 and 00001111. Moreover, $U$ should be restricted to only FOUR $X/Y$ Pauli Matrices. Two $X/Y$ in the occupied spin-orbital and two $X/Y$ in the non-occupied spin-orbitals.

- **Particle Number conservation ($\hat{N}$)**. If the number of $X/Y$ acting on "occupied" spin orbitals is different from the number of $X/Y$ acting on "non-occupied" (virtual) spin orbitals, then the number of particles is not conserved in the system

- **Total Spin and spin projection ($\hat{S}^2$ and $\hat{S}_z$)**. If the difference between the number of X/Y acting on alpha occupied orbitals and the number of X/Y acting on beta occupied orbitals, is equal to the difference between the number of X/Y acting on $\alpha$ non-occupied orbitals and the number of X/Y acting on $\beta$ non-occupied orbitals (or absolute value). Moreover, following the Jordan Wigner transformation [15], qubits are alternating between spin-up and spin-down orbitals such that the first, third, fifth, etc.., encode for spin-up, while the second, fourth, sixth, etc..., encode for spin-down. In the four-qubit case, an example of such a Pauli string is YIXI, which is spin symmetric as it contains two X or Y Pauli operators acting on the $\alpha$ orbitals and no operators acting on the $\beta$ orbitals. It should at the same time preserve the particle numbers.

- **Point group ($\hat{R}_i$)**. For a given symmetry operation $\hat{R}_i$ belonging to an Abelian point group, the Hamiltonian commutes with it: $[\hat{H}, \hat{R}_i] = 0$. This implies that when the symmetry operator acts on the wavefunction ($|\psi_0\rangle$)

of the Hamiltonian, the resulting wavefunction $|\Psi\rangle = \hat{R}_i|\psi_0\rangle$ is also an eigenstate of the system. The eigenvalue of $\hat{R}_i|\psi_0\rangle$ is expressed, as $\gamma|\psi_0\rangle$, where the value of $\gamma$ is an irreducible character, that can be looked up from the character table of the corresponding point group (see character tables for their associated point groups in reference [16]). The irreducible characters in the Abelian point group are always either 1 or -1. Our goal is to show that $|\psi_0\rangle$ and $|\psi\rangle$ belong to the same irreducible representation (denoted as *irrep*):
(i) by applying the symmetry on $|\psi\rangle$, then overlapping it with the symmetry acted on $|\psi_0\rangle$, we then have $\langle\psi_0|\hat{R}_i{}^\dagger\hat{R}_i|\psi\rangle = c_0c_1\langle\psi_0|\psi\rangle$. We note that a reasonable solution $|\psi\rangle$ perturbed from $|\psi_0\rangle$ should be overlapping with the Hartree-Fock determinant $|\psi_{HF}\rangle$, which indicates that $c_0c_1 = 1$. However, since in an Abelian group, $\gamma$ is either +1 or -1, $c_0$ must equal to $c_1$. So, in our case, the qubit excitations starters which generate the disentangled wavefunction, are required to have the same *irrep* as the reference wavefunction $|\psi_{HF}\rangle$. It indicates that the double excitations generated constrained by four X/Y Pauli, should belong to the corresponding irrep of the Hartree-Fock state, and consequently they can only survive in the selection process. Thus, in our algorithm, we filter out the excitation operators that belong to a different *irrep.* To illustrate this concept simply, we provide the following example. In a closed shell molecule, such as $BeH_2$, which consists of 6 electrons, there is balance between the three spin-up and three spin-down electrons, which indicates that the Hartree-Fock state of $BeH_2$ belongs to $A_g$ representation in the $D_{2h}$ Abelian point group. Then the *irrep* of the total wavefunction $|\Psi\rangle$ should be the same. To label the orbitals in terms of irreducible representations using the reference [16], we have

$$A^\alpha A^\beta A^\alpha A^\beta B^\alpha B^\beta C^\alpha C^\beta D^\alpha D^\beta A^\alpha A^\beta B^\alpha B^\beta.$$

Since the $BeH_2$ molecule has 14 qubits, the Hartree-Fock state acting on these qubits is represented as $|\psi_{HF}\rangle$ = $|11111100000000\rangle$, which actually belongs to $A$ irrep. Then, any excitation $\hat{P}$ would be symmetric and can be included in the set of starters, if and only if it belongs to same "$A$" final representation. For example $\hat{P}$ = ZYXIZZZZZYYIIII belongs to $A$ *irrep*, while $\hat{P}$ = ZYXIZZZZZYIIYII belongs to $B$ *irrep* and thus it should be filtered out because it does not respect the $\hat{R}_i$ symmetric operations on the Hartree-Fock state.

## 5. PERFORMANCES OF THE MCP GENERATION

In this section, evaluate the performances of the C++ MCP generation subroutine, evaluating memory and time consumption as the number of qubits increases. The reader should refer to the Figures below for details.

When comparing the performance of the Python and C++ implementations of the [17], several critical factors come into play in the context of High-Performance Computing (HPC): execution speed, memory consumption, and ease of optimization.

- **Execution Speed** C++ is generally much faster than Python due to its nature as a compiled language. In C++, a code is compiled into machine language, which the computer's CPU can execute directly. This results in very fast execution times because the overhead of interpretation is eliminated. Additionally, C++ offers fine-grained control over hardware and memory management, enabling developers to optimize performance at a very low level.

  Python, on the other hand, is an interpreted language. Python code is executed by an interpreter, which introduces significant overhead because the code must be parsed and executed line by line. While Python has implementations like PyPy that offer Just-In-Time (JIT) compilation to improve performance, it still generally lags behind C++ in raw execution speed.

- **Memory Consumption** Memory management in C++ is manual, allowing developers to allocate and deallocate memory precisely. This control can be advantageous in HPC environments where memory efficiency is critical. Developers can optimize memory usage to reduce overhead and ensure that large datasets are handled efficiently. C++ also supports low-level data structures and operations that can be tailored to use minimal memory.

  Python handles memory management automatically through its garbage collection system. While this simplifies development by reducing the risk of memory leaks, it can lead to higher memory consumption and less predictability in memory usage. Python's data structures are more abstracted, which can introduce additional memory overhead. In our case, storing the FullGroup in python as a python set is memory consuming when we try to scale up. We designed a specific C++ data structure set that minimizes memory consumption to the detriment of searching operations in order to be able to hold large set and increase the number of qubits. This

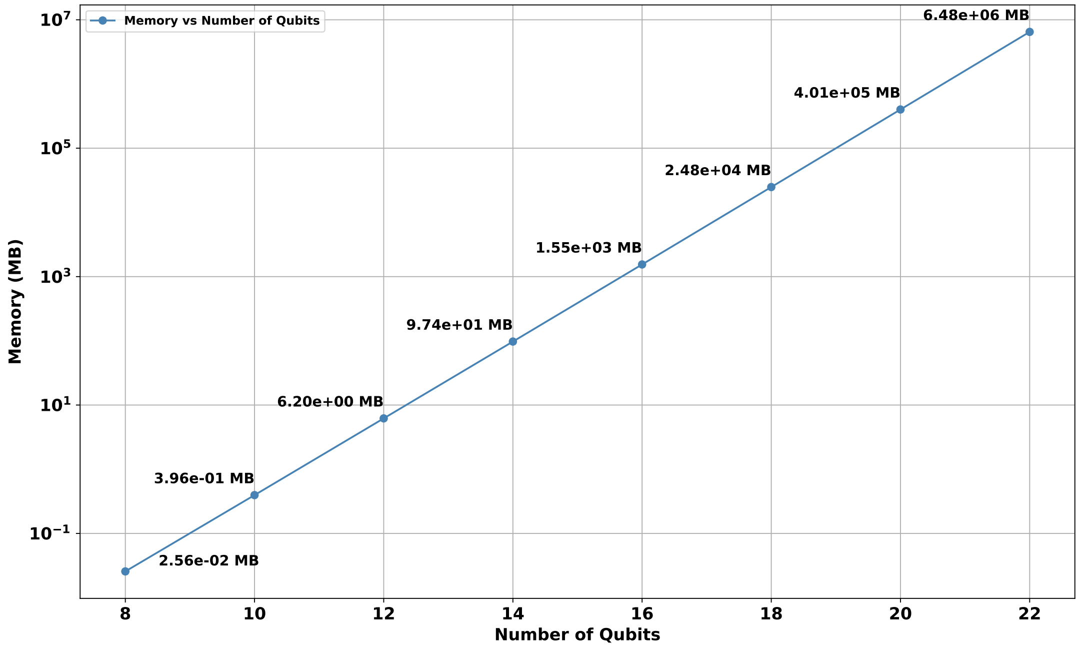


(a) Memory use

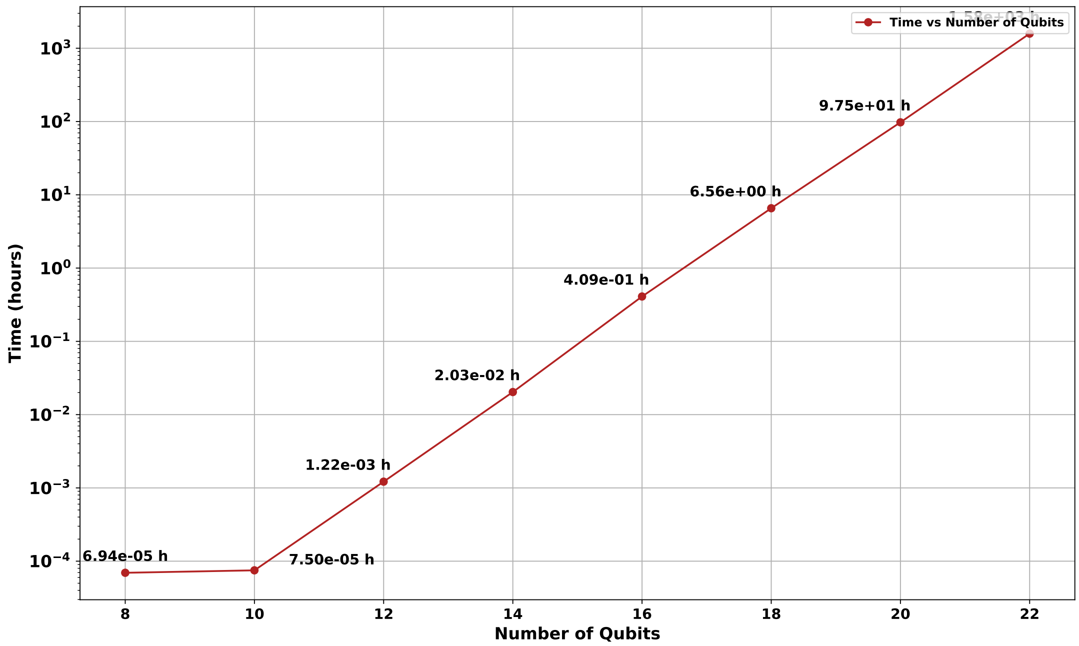


(b) Timings

FIG. S3: (a) Memory usage and (b) timings for generating an MCP while increasing the number of qubits, implemented in "optimized" version C++ compilation, and, measured using standard computer machine described in the main text.

grants the ability to run 14 qubits 7 electrons MCP Build on a laptop without suffering from memory issues; since it only requires now 500 MiB compares to the 14 GiB from the python code.

- **Time to Solution** Python excels in terms of development speed and time to solution. Its high-level syntax and extensive libraries make it easier and faster to write and maintain code. This rapid development cycle is particularly beneficial in research and prototyping phases of HPC projects, where flexibility and ease of iteration

are crucial.

C++, however, requires more time to write and debug due to its complexity and the need for detailed memory management. Although it may take longer to develop an initial solution in C++, the resulting code is typically more efficient and better suited for production environments where performance is paramount.

- **HPC Optimization** In HPC, optimization at the hardware level is critical. C++ allows developers to utilize advanced optimization techniques such as SIMD (Single Instruction, Multiple Data), parallel processing with OpenMP (use in our case when assembling the starters and FullSet) or MPI, and hardware-specific optimizations that can drastically improve performance. Presently, we only used OpenMP, as MPI and GPU will be considered in further work in the context of the Hyperion-1 GPU-accelerated emulator.[18]

Note that a GPU portage would not solve by itself the issue of the exponential growth that arises from construction the MCP. Indeed, beside the speed of execution, the memory will remain the main bottleneck on GPUs as we estimate an amount of 8Tb to construct a 22 qubits MCP.

Python's optimization capabilities are more limited. While there are libraries like NumPy and tools like python that enable some level of optimization, they cannot match the low-level control and performance tuning possible with C++. For instance, NumPy is implemented in C, allowing Python to leverage C's performance indirectly, but this still introduces some overhead.


[1] M. Hjorth-Jensen, Second quantization (2015), http://nucleartalent.github.io/Course2ManyBodyMethods/doc/pub/secondquant/html/secondquant-bs.html, Last accessed on 2024-07-05.
[2] H. R. Grimsley, S. E. Economou, E. Barnes, and N. J. Mayhall, An adaptive variational algorithm for exact molecular simulations on a quantum computer, Nature communications **10**, 1 (2019).
[3] H. L. Tang, V. Shkolnikov, G. S. Barron, H. R. Grimsley, N. J. Mayhall, E. Barnes, and S. E. Economou, qubit-adapt-vqe: An adaptive algorithm for constructing hardware-efficient ansätze on a quantum processor, PRX Quantum **2**, 020310 (2021).
[4] Y. S. Yordanov, V. Armaos, C. H. Barnes, and D. R. Arvidsson-Shukur, Qubit-excitation-based adaptive variational quantum eigensolver, Communications Physics **4**, 228 (2021).
[5] J. Liu, Z. Li, and J. Yang, An efficient adaptive variational quantum solver of the schrödinger equation based on reduced density matrices, The Journal of chemical physics **154** (2021).
[6] P. G. Anastasiou, Y. Chen, N. J. Mayhall, E. Barnes, and S. E. Economou, Tetris-adapt-vqe: An adaptive algorithm that yields shallower, denser circuit ans\" atze, arXiv preprint arXiv:2209.10562 (2022).
[7] V. O. Shkolnikov, N. J. Mayhall, S. E. Economou, and E. Barnes, Avoiding symmetry roadblocks and minimizing the measurement overhead of adaptive variational quantum eigensolvers, Quantum **7**, 1040 (2023).
[8] C. Feniou, M. Hassan, D. Traoré, E. Giner, Y. Maday, and J.-P. Piquemal, Overlap-adapt-vqe: Practical quantum chemistry on quantum computers via overlap-guided compact ans\" atze, arXiv preprint arXiv:2301.10196 (2023).
[9] D. A. Fedorov, Y. Alexeev, S. K. Gray, and M. Otten, Unitary selective coupled-cluster method, Quantum **6**, 703 (2022).
[10] D. Mondal, D. Halder, S. Halder, and R. Maitra, Development of a compact ansatz via operator commutativity screening: Digital quantum simulation of molecular systems, The Journal of Chemical Physics **159** (2023).
[11] D. Halder, D. Mondal, and R. Maitra, Noise-independent route toward the genesis of a COMPACT ansatz for molecular energetics: A dynamic approach, The Journal of Chemical Physics **160**, 124104 (2024), https://pubs.aip.org/aip/jcp/article-pdf/doi/10.1063/5.0198277/19844810/124104_1_5.0198277.pdf.
[12] S. McArdle, S. Endo, A. Aspuru-Guzik, S. C. Benjamin, and X. Yuan, Quantum computational chemistry, Reviews of Modern Physics **92**, 015003 (2020).
[13] J. D. Whitfield, J. Biamonte, and A. Aspuru-Guzik, Simulation of electronic structure hamiltonians using quantum computers, Molecular Physics **109**, 735 (2011).
[14] C. Hempel, C. Maier, J. Romero, J. McClean, T. Monz, H. Shen, P. Jurcevic, B. P. Lanyon, P. Love, R. Babbush, *et al.*, Quantum chemistry calculations on a trapped-ion quantum simulator, Physical Review X **8**, 031022 (2018).
[15] E. Fradkin, Jordan-wigner transformation for quantum-spin systems in two dimensions and fractional statistics, Physical review letters **63**, 322 (1989).
[16] P. W. Atkins, M. S. Child, and C. S. G. Phillips, *Tables for group theory*, Vol. 6 (Oxford University Press Oxford, 1970).
[17] V. Shkolnikov, Code used to generate minimal complete pool and find the ground state of lithium hydrid, https://github.com/VladShkolnikov/H4_dissociation_curve/blob/main/H4_pool_construct.ipynb.
[18] O. Adjoua, C. Feniou, and et al., Sorbonne Université, CNRS and Qubit Pharmaceuticals (2024).
